# Supplementary material for: Finite-Blocklength Performance of Sequential Transmission over BSC with Noiseless Feedback
Source: arXiv:1902.00593 source file (2020-05-28)
Supplement: Supplementary file 1 [file last_stage.tex]

\documentclass{article}

\usepackage[margin=0.2in]{geometry}
\usepackage{tikz}
\usepackage{amsmath}
\usepackage{amssymb}
\usetikzlibrary{arrows,decorations.pathmorphing,backgrounds,positioning,fit,petri,shapes}

\newcommand{\St}{\mathcal{S}}

\begin{document}
\thispagestyle{empty}
\tikzpicture
	[every place/.style={ellipse,minimum size=10mm,inner sep=0pt},
	pre/.style={<-,shorten <=1pt,>=stealth',very thick},
	post/.style={->,shorten <=1pt,>=stealth',very thick},
	information text/.style={rounded corners,fill=black!10,inner sep=1ex},
	auto,scale=1]
	
	\node [place,label=below: $\St_{n-1}$] (sE) at (10.6,1) {$u^*+$\\ $(n-1)C_2$}
		edge [pre,in=160,out=200,loop] node {$p$} (sE);
	\node [place,label=below: $\St_n$] (EXIT)	at (14.5,1) {$u^*+nC_2$}
		edge [pre, bend right]					node [swap]{$q$}	(sE)
		edge [pre, in=340,out=20,loop] node {$1$} (EXIT);
\endtikzpicture

\end{document}
